# Supplementary material for: All Byzantine Agreement Problems are Expensive
Source: arXiv:2311.08060 source file (2023-11-15)
Supplement: Supplementary file 1 [file triviality_proof.tex]

\section{Triviality of Unauthenticated-Solvable Agreement Problems}

In this section, we formally prove the following theorem:

\begin{theorem} \label{theorem:unauthenticated_triviality}
If a Byzantine agreement problem is unauthenticated-solvable with $n \leq 3t$, the problem is trivial, i.e., there exists a value $v' \in \bigcap\limits_{c \in \mathcal{I}} \mathit{val}(c)$.
\end{theorem}

To prove \Cref{theorem:unauthenticated_triviality}, we first show that no non-trivial Byzantine agreement problem is unauthenticated-solvable with $n = 3$ and $t = 1$ (\Cref{subsection:three_processes}).
Then, we extend the result to any $n$ and $t$ with $n \leq 3t$.

\subsection{Triviality with Three Processes} \label{subsection:three_processes}

This subsection proves the following theorem:

\begin{theorem} \label{theorem:three_processes}
If any Byzantine agreement problem is unauthenticated-solvable with $n = 3$ and $t = 1$, the problem is trivial.
\end{theorem}

We prove \Cref{theorem:three_processes} by contradiction.
Namely, we assume that there exists a non-trivial Byzantine agreement problem $\mathit{val}$-agreement which is unauthenticated-solvable with $n = 3$ and $t = 1$; moreover, we fix $\mathcal{A}$, any unauthenticated algorithm which solves $\mathit{val}$-agreement.
Furthermore, throughout the proof, we fix the following parameters:
\begin{compactitem}
    \item We fix any proposal $v \in \mathcal{V}_I$.
    
    \item We fix any input configuration $c_1 \in \mathcal{I}_3$ such that (1) $\pi(c_1) = \Pi$, and (2) $\mathit{proposal}(c_1[1]) = \mathit{proposal}(c_1[2]) = \mathit{proposal}(c_1[3]) = v$.

    \item We fix the infinite execution $\mathcal{E}_1$ such that $\mathsf{input\_conf}(\mathcal{E}_1) = c_1$.
    As $\mathcal{A}$ satisfies \emph{Termination} and \emph{Agreement}, some value $v_1' \in \mathcal{V}_O$ is decided in $\mathcal{E}_1$. 

    \item We fix any input configuration $c_2^* \in \mathcal{I}$ such that $v_1' \notin \mathit{val}(c_2^*)$.
    (Observe that such an input configuration exists since $\mathit{val}$-agreement is non-trivial.)

    \item We fix the input configuration $c_2 \in \mathcal{I}_3$ such that the following holds:
    \begin{compactitem}
        \item for every $P_i \in \pi(c_2^*)$, $c_2[i] = c_2^*[i]$, and

        \item for every $P_i \notin \pi(c_2^*)$, $\mathsf{proposal}(c_2[i]) = v$.
    \end{compactitem}
    Note that $c_2 \rhd c_2^*$.

    \item We fix the infinite execution $\mathcal{E}_2$ such that $\mathsf{input\_conf}(\mathcal{E}_2) = c_2$.
    As $\mathcal{A}$ satisfies \emph{Termination} and \emph{Agreement}, some value $v_2' \in \mathcal{V}_O$ is decided in $\mathcal{E}_2$. 
\end{compactitem}

In summary, we prove \Cref{theorem:unauthenticated_triviality} by pairing (1) the celebrated ``hexagon'' proof-technique~\cite{lynch1996distributed,FischerLM85}, with (2) the fact that $v_1' \neq v_2'$, which we prove below.

\begin{lemma} \label{lemma:neq}
$v_1' \neq v_2'$.
\end{lemma}
\begin{proof}
By contradiction, let $v_1' = v_2'$.
Recall that $c_2 \rhd c_2^*$.
Thus, \Cref{lemma:canonical_containment} states that $v_1' \in \mathit{val}(c_2^*)$, which represents a contradiction.
\end{proof}

Let $r_1$ denote the smallest round number by which all processes decide $v_1'$ in $\mathcal{E}_1$.
Similarly, let $r_2$ denote the smallest round number by which all processes decide $v_2' \neq v_1'$ in $\mathcal{E}_2$.
Let $r \geq \max(1, r_1, r_2)$.
Following the ``hexagon'' proof-technique, we construct a new system $\mathcal{S}$ by copying $2r$ copies of the algorithm $\mathcal{A}$ into a ring with $6r$ processes: $3r$ in the upper part, and $3r$ in the lower part of the ring.
Each process $P_i \in \Pi$ has $r$ copies in $\mathcal{S}$ and each process which is in the ring correctly follows $\mathcal{A}$.
In the upper part, each process $P_i$ starts with the proposal $v$.
In the lower part, each process $P_i$ starts with the proposal $\mathsf{proposal}(c_2[i])$.
The exact depiction of $\mathcal{S}$ is given in \Cref{fig:ring}.
Let the described execution of the described system $\mathcal{S}$ be denoted by $\mathcal{E}_{\mathcal{S}}$.
The following lemma proves that any two processes adjacent in $\mathcal{S}$ decide the same value in $\mathcal{E}_{\mathcal{S}}$.
% As the following lemma is well-known in the literature (see~\cite{lynch1996distributed,FischerLM85}), we provide an informal proof for completeness.

\begin{lemma} \label{lemma:adjacent}
Any two processes which are adjacent in $\mathcal{S}$ decide the same value in $\mathcal{E}_{\mathcal{S}}$.
\end{lemma}
\begin{proof}
See~\cite{lynch1996distributed}.
\end{proof}

\Cref{lemma:adjacent} implies that all processes in $\mathcal{S}$ must decide the same value:

\begin{corollary} \label{corollary:all_same}
All processes in $\mathcal{S}$ decide the same value in $\mathcal{E}_{\mathcal{S}}$.
\end{corollary}
